# Supplementary material for: Duality and degeneracy lifting in two-dimensional electron liquids on SrTiO$_3$(001)
Source: arXiv:2405.18946 ancillary file (2024-05-31)
Supplement: Supplementary file 1 [file Supplement_Duality_and_Degeneracy_Lifting_in_2DELS_on_SrTiO3_001.pdf]

# SUPPLEMENTAL MATERIAL

## Duality and degeneracy lifting in two-dimensional electron liquids on SrTiO<sub>3</sub>(001)

Igor Sokolović,<sup>1</sup> Eduardo B. Guedes,<sup>2</sup> Thomas P. van Waas,<sup>3</sup> Samuel Poncé,<sup>3,4</sup> Craig Polley,<sup>5</sup> Michael Schmid,<sup>1</sup> Ulrike Diebold,<sup>1</sup> Milan Radović,<sup>2</sup> Martin Setvín,<sup>1,6</sup> and J. Hugo Dil<sup>7,2</sup>

<sup>1</sup>*Institute of Applied Physics, TU Wien, 1040 Vienna, Austria*

<sup>2</sup>*Photon Science Division, Paul Scherrer Institut, CH-5232 Villigen, Switzerland*

<sup>3</sup>*European Theoretical Spectroscopy Facility, Institute of Condensed Matter and Nanosciences, Université catholique de Louvain, Chemin des Étoiles 8, B-1348 Louvain-la-Neuve, Belgium*

<sup>4</sup>*WEL Research Institute, Avenue Pasteur 6, 1300 Wavre, Belgium*

<sup>5</sup>*MAX IV Laboratory, Lund University, Lund, Sweden*

<sup>6</sup>*Department of Surface and Plasma Science, Faculty of Mathematics and Physics, Charles University, 180 00 Prague 8, Czech Republic*

<sup>7</sup>*Institut de Physique, École Polytechnique Fédérale de Lausanne, CH-1015 Lausanne, Switzerland*

### CONTENTS

|                                                                          |    |
|--------------------------------------------------------------------------|----|
| SM1. Identification of the surface terminations with SEM                 | 2  |
| SM2. Badly defined Fermi-surface maps                                    | 5  |
| SM3. Analysis of momentum distribution curves                            | 6  |
| SM4. Synchrotron-based XPS                                               | 7  |
| SM5. Photoemission matrix element correction                             | 9  |
| SM6. Bare band parameters                                                | 12 |
| SM7. Eliashberg spectral function analysis                               | 14 |
| SM8. Splitting of the $d_{xy}$ bands on the TiO <sub>2</sub> termination | 17 |
| SM9. Video captions                                                      | 19 |
| References                                                               | 20 |

### SM1. IDENTIFICATION OF THE SURFACE TERMINATIONS WITH SEM

Superposition of the lateral coordinates of the ARPES measurement positions onto the SEM image in Fig. 1c showed that the two distinct 2DELs appear on different terminations. Namely, the different FS maps lie on surface regions with different secondary electron contrast. To reveal which SEM contrast on a well-cleaved surface corresponds to which surface termination, we studied three separate cleaved  $\text{SrTiO}_3(001)$  crystals. Each was first investigated with atomic precision using in-situ ncAFM after cleaving, and subsequently measured with SEM ex situ. The results are summarized in Figs. SM1–SM3.

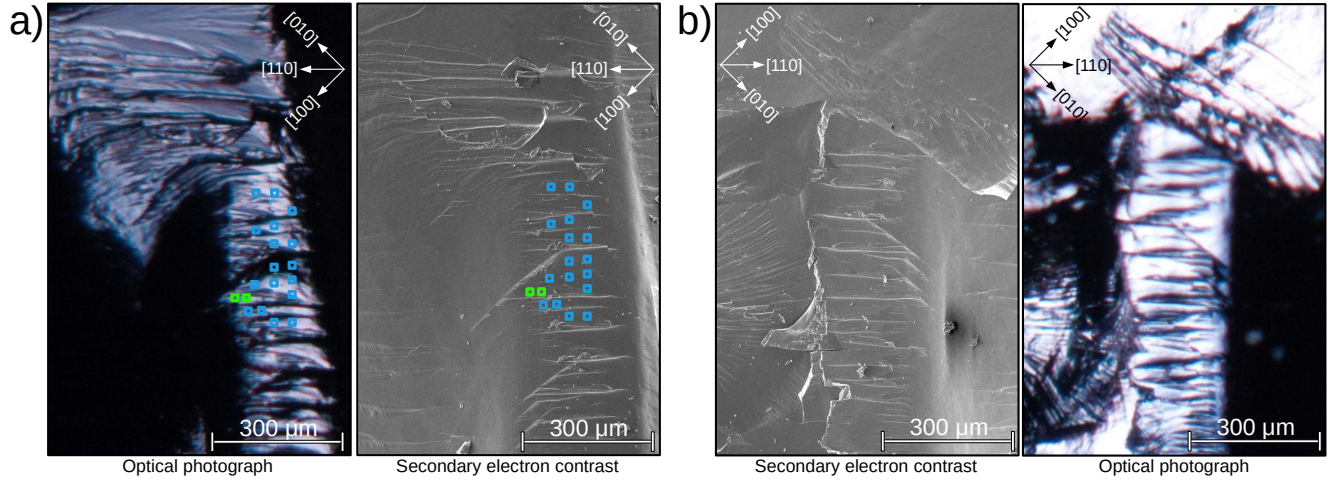

FIG. SM1. Optical photographs and secondary electron SEM images of two pieces of a  $\text{SrTiO}_3(001)$  surface cleaved in UHV and studied with microscopy: a) the piece that was investigated with ncAFM and STM to discern the rough spatial distribution of the two surface terminations and b) the mirror-symmetric counter-piece of the surface removed upon cleavage. Regions where  $\text{TiO}_2$  termination was observed with ncAFM in UHV are marked by blue squares, while regions where  $\text{SrO}$  termination was observed with ncAFM in UHV are marked by green squares. Optical photographs and the SEM images on the same side of the cleavage show the same surface regions. Crystallographic directions are indicated in each image.

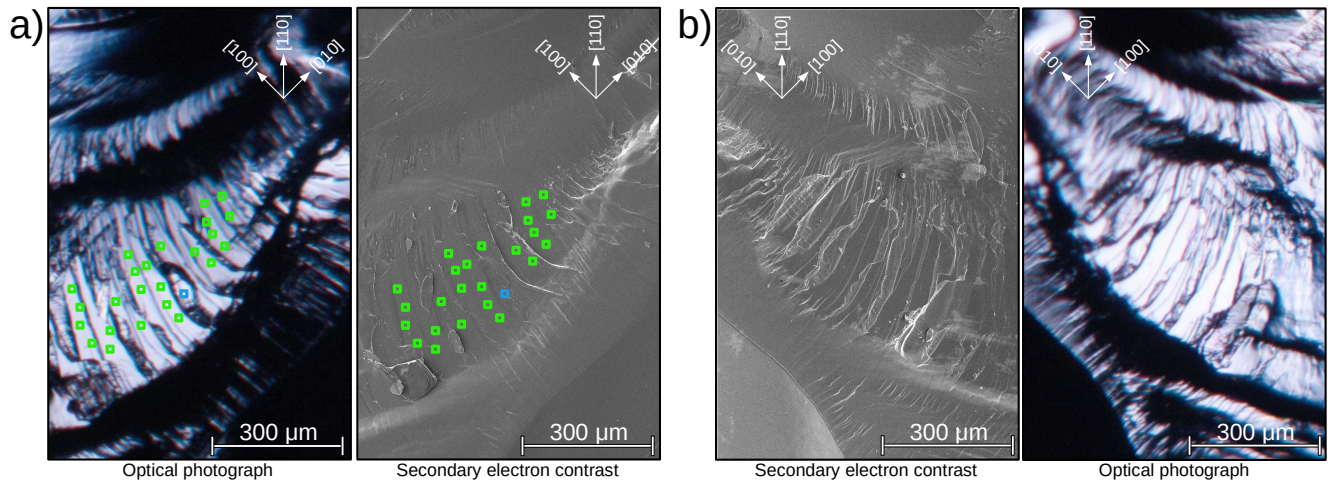

FIG. SM2. Optical photographs and secondary electron SEM images of two pieces of another  $\text{SrTiO}_3(001)$  surface cleaved in UHV and studied with microscopy: a) the piece that was investigated with ncAFM and STM to discern the rough spatial distribution of the two surface terminations and b) the mirror-symmetric counter-piece of the surface removed upon cleavage. Regions where  $\text{TiO}_2$  termination was observed with ncAFM in UHV are marked by blue squares, while regions where  $\text{SrO}$  termination was observed with ncAFM in UHV are marked by green squares. Optical photographs and the SEM images on the same side of the cleavage show the same surface regions. Crystallographic directions are indicated in each image.

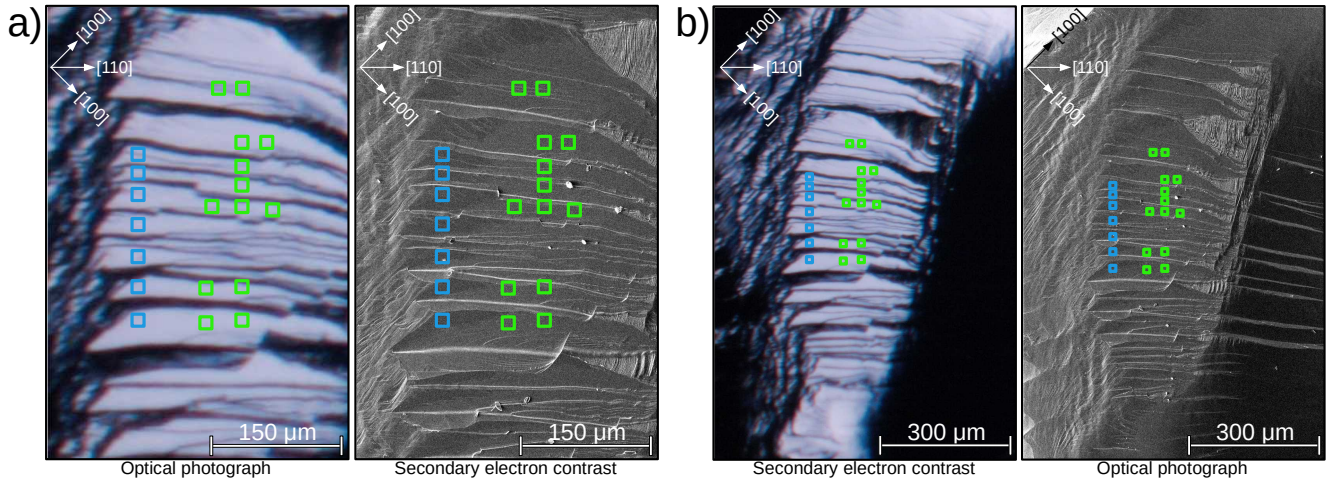

FIG. SM3. Optical photographs and secondary electron SEM images of the a third  $\text{SrTiO}_3(001)$  surface cleaved in UHV and studied with microscopy displayed in: a) large magnification and b) smaller magnification. Regions where  $\text{TiO}_2$  termination was observed with ncAFM in UHV are marked by blue squares, while regions where SrO termination was observed with ncAFM in UHV are marked by green squares. Optical photographs and the SEM images side-by-side show roughly the same surface regions. Crystallographic directions are indicated in each image.

For each sample in Figs. SM1–SM3 only one side of the cleaved  $\text{SrTiO}_3(001)$  was studied with ncAFM. Each of these surfaces was investigated at many different lateral positions on a well-cleaved surface patch, and atomic resolution was used to discern whether each point was  $\text{TiO}_2$ - or SrO-terminated. These surfaces and their mirror-symmetric counterparts were then photographed with high magnification. The positions investigated with ncAFM were superimposed on these optical photographs as blue and green squares where the surface was observed to be  $\text{TiO}_2$ - or SrO-terminated, respectively. Both the investigated  $\text{SrTiO}_3(001)$  surfaces and their respective counterparts were subsequently imaged with SEM to discern the spatial distribution of the terminations (Figs. SM1–SM2), with one exception (Fig. SM3), where the mirror-symmetric counterpart to the investigated surface was unfortunately lost before optical and SEM images could be taken.

On  $\text{SrTiO}_3(001)$  surfaces studied in Fig. SM1, ncAFM measurements on one side of the cleavage (Fig. SM1a) indicated that this particular surface region is predominantly  $\text{TiO}_2$ -terminated. Many positions across the terrace train were investigated, and only two times out of approximately 20 times the surface exposed the SrO termination, which occurred in two positions that are laterally close to each other. In SEM, the majority of this terrace train displays dark contrast (Fig. SM1a), while only a small portion of this surface region (close to the “left” border) displays a bright signal. This means that the  $\text{TiO}_2$  termination is imaged as dark with SEM. The mirror-symmetric part of this cleavage (Fig. SM1b) showed the opposite contrast: The majority of the terrace train is visible in bright contrast. As this side of the cleavage must have the opposite termination – SrO in this case – it implies that the SrO is seen as bright contrast in SEM.

A similar distribution of surface terminations was observed in the second sample, shown in Fig. SM2. There, the majority of the surface studied in vacuum with ncAFM turned out to be SrO-terminated (Fig. SM2a). The SEM contrast shows that the majority of this surface region is bright and not particularly distinguishable from the surrounding conchoidal fracture. The other side of this cleavage (Fig. SM2b) shows the opposite SEM contrast: The majority of atomically flat terraces are imaged with the dark contrast. As the mirror-symmetric part of the cleavage must be  $\text{TiO}_2$ -terminated, it is established that the bright SEM contrast corresponds to the SrO, while the dark SEM contrast corresponds to the  $\text{TiO}_2$  termination.

Finally, on the third sample, seen in Fig. SM3 with two different optical and SEM magnifications, ncAFM measurements showed that both surface terminations are present on the selected well-cleaved surface region. Many regions close to the left border of the well-cleaved surface patch were found to be pre-dominantly  $\text{TiO}_2$ -terminated, while the surface areas closer to the right border were observed to be the SrO termination. Optical photographs cannot distinguish between these two terminations, but the SEM clearly indicates that the region close to the left border has significant dark patches, while the region close to the right border is predominantly bright:  $\text{TiO}_2$  was again measured as dark and the SrO as bright SEM contrast.

All three  $\text{SrTiO}_3(001)$  cleavages in Figs. SM1–SM3 consistently demonstrated that the  $\text{TiO}_2$  termination can be recognized as dark and the SrO termination can be recognized as bright in the SEM contrast. The mirror-symmetric

$\text{SrTiO}_3(001)$  surface has an opposite contrast. This knowledge was applied to the sample investigated under synchrotron light in Fig. 1c of the main text, to recognize which of the two well-defined 2DELs correspond to which termination.

It is important to emphasize that the SEM image in Fig. 1c of the main text was taken on the mirror-symmetric counterpart of the surface actually studied with synchrotron-based ARPES, because the ARPES-investigated surface was lost during transport between to the SEM. Therefore, Fig. 1c of the main text shows the positions corresponding to the ARPES measurements on the images of the cleaving counterpart. This means that the SEM contrast of the  $\text{TiO}_2$  and  $\text{SrO}$  surfaces is inverted with respect to the sample measured by ARPES. To summarize:

- The double-ringed Fermi surfaces are located on bright SEM contrast on the mirror-symmetric cleaved surface in Fig. 1c, which means that the double-ringed Fermi surface corresponds to dark SEM contrast on the actual surface where the ARPES measurements took place, i.e., on the  $\text{TiO}_2$  termination.
- The single-ringed Fermi surfaces are located on dark SEM contrast on the mirror-symmetric cleaved surface in Fig. 1c, which means that the single-ringed Fermi surface corresponds to bright SEM contrast on the actual surface where the ARPES measurements took place, i.e., on the  $\text{SrO}$  termination.

## SM2. BADLY DEFINED FERMI-SURFACE MAPS

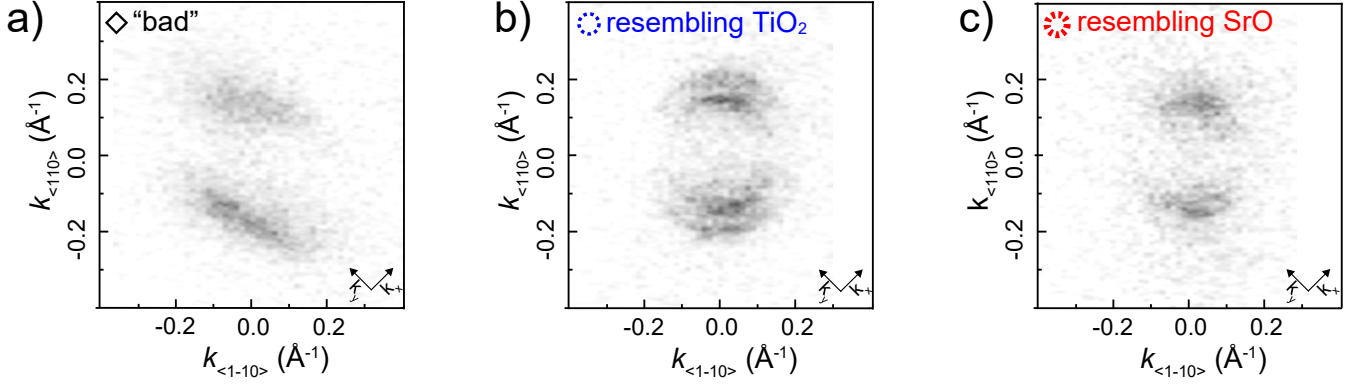

FIG. SM4. Fermi surface maps that do not show a structure as clear as the ones shown in the main text. These maps were obtained on surface regions marked by a) black diamonds, b) blue broken circles, and c) red broken circles in Fig. 1c of the main text.

Figures 1e and 1f of the main text show representative FS maps repeatedly obtained on well-cleaved  $\text{SrTiO}_3(001)$  surface regions with a known atomic structure. Several different FS maps were observed on the locations marked in Fig. 1c of the main text with black diamonds, and blue and red broken circles. Representative measurements of these FSs are shown here in Fig. SM4 for completeness.

The worst FS maps were obtained on regions marked as black diamonds in Fig. 1c of the main text and one such FS can be seen in Fig. SM4a. They are characterized by an ill-defined intensity distribution along the reciprocal lattice vectors and a clear absence of inversion symmetry. We assign these FS maps as being taken on a surface region with a high density of morphological defects such as dislocations, step bunching, and macroscopic cracks in the bulk.

Fermi surface maps that resemble the 2DELs respectively formed on  $\text{TiO}_2$ - and  $\text{SrO}$ -terminated surfaces are shown in Figs. SM4b and SM4c, which correspond to measurement positions marked with broken blue and broken red circles in Figs. 1e and 1f of the main text. These FS maps are better defined than those obtained on surface regions dominated by morphological defects (Fig. SM4a) and possess a clear structure, which could be described as a combination of the two well-defined FSs in Fig. 1c of the main text. We attribute these FS to correspond at surface regions with mixed surface terminations. This mixing can originate from either (i) measuring at positions where the synchrotron beam covers the transition between the two terminations, i.e., across a domain wall on the well-cleaved surface regions, or (ii) measuring at the surface areas with conchoidal fracture, i.e., with an ill-defined atomic structure.

### SM3. ANALYSIS OF MOMENTUM DISTRIBUTION CURVES

As explained in the main text, the difference between the 2DELs found in the  $\text{TiO}_2$ - and  $\text{SrO}$ -terminated surfaces cannot be attributed to a spectral broadening. To illustrate this fact, Fig SM5 shows the MDC at  $E_F$  along the  $\langle 110 \rangle$  direction of the  $\text{TiO}_2$ -terminated surface, as well as the same data convolved with Gaussian profiles of different FWHM, from 0.001 to 0.02  $\text{\AA}^{-1}$ . Compared with an equivalent MDC of the  $\text{SrO}$ -terminated surface, it becomes clear that the spectral distribution arising from the  $\text{TiO}_2$ -terminated surface cannot evolve into the  $\text{SrO}$ -terminated one simply via broadening.

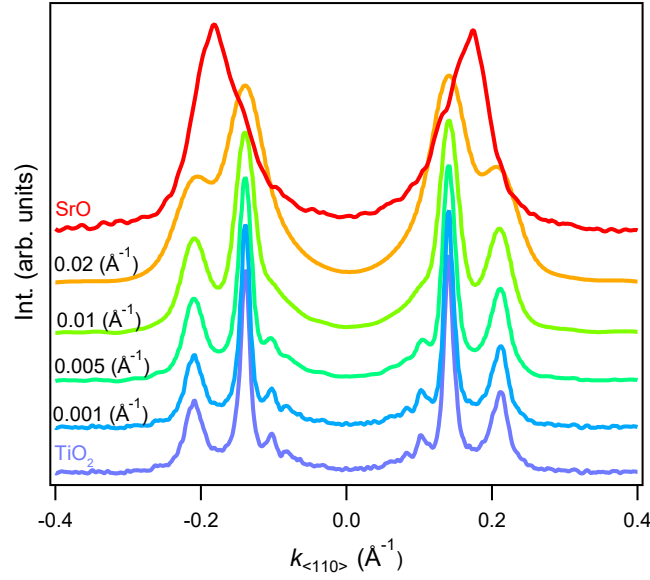

FIG. SM5. Momentum distribution curves at  $E_F$  of the  $\text{TiO}_2$ -terminated surface as measured and convolved with Gaussian profiles of different full width at half maximum, compared with the  $\text{SrO}$ -terminated surface.

## SM4. SYNCHROTRON-BASED XPS

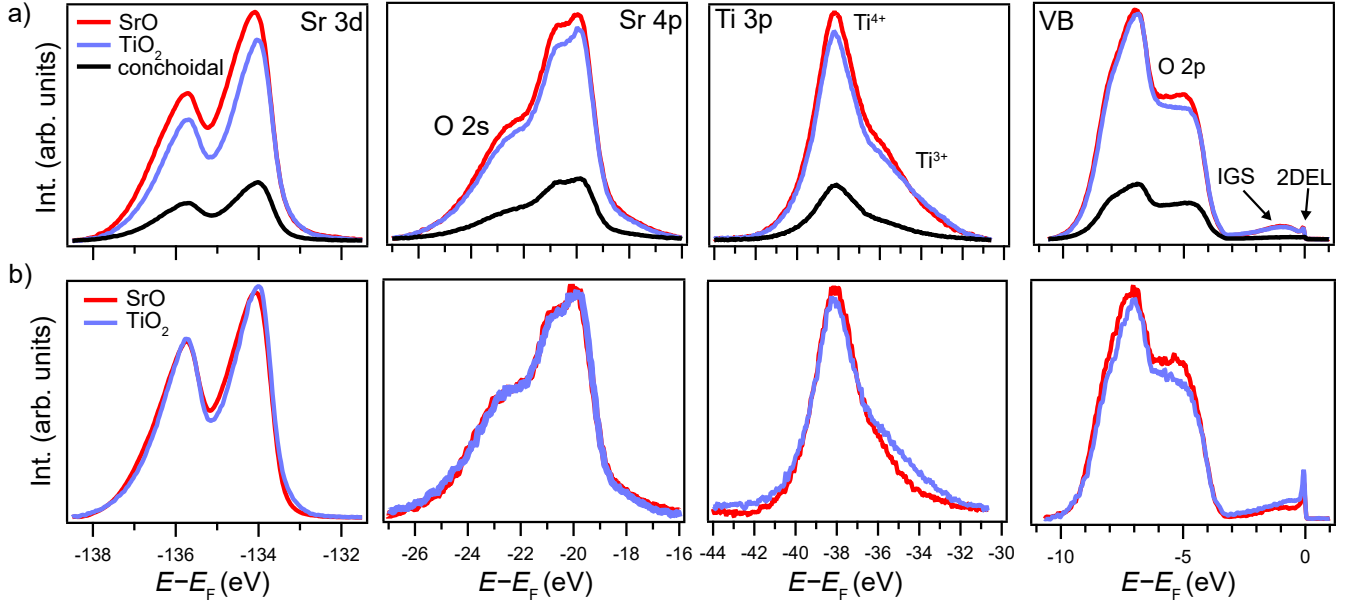

FIG. SM6. XPS measurements of three shallow core levels and the top of the valence band measured by irradiation of the cleaved surface with synchrotron light with a photon energy of a)  $h\nu = 170$  eV and b)  $h\nu = 230$  eV. XPS measurements over surface regions where a badly defined Fermi surface was observed (black diamonds in Fig 1c) are shown in black.

The chemical composition of the two terminations was investigated in situ by synchrotron based X-ray photoelectron spectroscopy (XPS) measurements, shown in Fig. SM6, using  $h\nu = 170$  eV and  $h\nu = 230$  eV. The subpanels show the spectra measured on surface areas that exhibited a double-ringed FS corresponding to the  $\text{TiO}_2$  termination (blue); a single-ringed FS corresponding to the  $\text{SrO}$  termination (red); and an ill-defined FS (only for  $h\nu = 170$  eV; black). A Shirley-type background was removed from all the spectra, and no further treatment was performed.

The XPS spectra obtained at different positions are very similar. This result is not surprising as the two surface terminations differ in only one atomic layer, while the “bad” surface regions are a combination of the two terminations. Moreover, both terminations on a well-cleaved surface region host intrinsic point defects inherent to the opposite termination:  $\text{TiO}_2$  has  $\approx 14\%$  excess Sr adatoms and  $\text{SrO}$  has  $\approx 14\%$  missing Sr atoms in the form of Sr vacancies. Therefore, the differences in the elemental compositions of the two terminations could be reasonably distinguished if the XPS probing depth in Fig. SM6 was one atomic layer only: the ratio of Sr atoms on the  $\text{SrO}$  and  $\text{TiO}_2$  termination would be  $86/14 = 6.14$  (without taking into account the interference effects and forward focusing of the photoelectrons). However, the probing depth was obviously not a single atomic layer as the Ti signal is present on both terminations. With an increase in the probing depth, the distinction between the two terminations becomes less evident. However, slight differences are still noticeable and are discussed below.

A prominent distinction between XPS spectra obtained on different surface terminations in Fig. SM6 is a slight shift of the  $\text{Sr } 3d$  and  $\text{Sr } 4p$  core levels on the  $\text{TiO}_2$  termination towards lower kinetic energies, i.e., higher binding energies. This shift is an indicator of an under-coordinated Sr adatoms on the  $\text{TiO}_2$  termination, intrinsic to the as-cleaved surface: the ionic cores of under-coordinated  $\text{Sr}^{2+}$  atoms are screened less efficiently, and all Sr electrons are therefore subjected to a higher binding energy.

The core levels of the Ti atoms are centered at the same energy, without detectable chemical shifts caused by under-coordination. That is to be expected as only the Sr atoms/vacancies act as a polarity compensating mechanism. There are noticeable differences in the Ti core level taken at different terminations mainly in the intensity and the energy distribution of the  $\text{Ti}^{3+}$  states. The  $\text{TiO}_2$  termination apparently hosts more  $\text{Ti}^{3+}$  atoms with bound charges, especially when probed with higher photon energy (Fig. SM6b).

The top of the valence band, right before the onset of the band gap, of the  $\text{TiO}_2$  termination is distinctly different from the  $\text{SrO}$  termination and the ill-defined conchoidal fracture. While we have shown that 2DEL develops on  $\text{SrO}$  through the formation of oxygen vacancies (Fig. 3 of the main text), it is expected that the conchoidal fracture develops a 2DEL in a similar fashion, as it was observed that it appears in a comparable time frame to the one on

the SrO termination (not shown). The well-cleaved  $\text{TiO}_2$  termination is the only place on a cleaved  $\text{SrTiO}_3(001)$  that hosts a 2DEL without the necessity of creating oxygen vacancies, that are additionally unfavorable on this termination (no observed defects with ncAFM). In that light, these differences in the top of the valence band could indicate that the  $\text{TiO}_2$  termination in fact does not develop oxygen vacancies during prolonged synchrotron irradiation. In this context it is important to reiterate that the  $\text{Ti}^{3+}$  states are related to trapped electrons and not necessarily to oxygen vacancies.

### SM5. PHOTOEMISSION MATRIX ELEMENT CORRECTION

In this section, we discuss the choice of the photoemission matrix element correction used to fit the  $d_{xy}$  bands and provide further details on the dispersions and electron self-energies extracted from the  $h\nu \in \{47 \text{ eV}, 85 \text{ eV}\}$  band maps for both types of surface terminations. We consider the electron self-energy  $\Sigma_n(E, \mathbf{k})$  for a band  $n$ , electron energy  $E$ , and momentum  $\mathbf{k}$  from ARPES. Since we only extract the Eliashberg function  $\alpha^2 F_n(\omega, \mathbf{k})$  for the outer band and phonon energy  $\omega$ , we drop the band index  $n$ , writing  $\Sigma(E, \mathbf{k})$  and  $\alpha^2 F(\omega, \mathbf{k})$ . Considering phonons (ph) as the only relevant bosonic species, the total electron self-energy for a weakly correlated system can be decomposed into its respective impurity (im), electron (el), and phonon contributions, according to Matthiessen's rule [1]:

$$\Sigma(E, \mathbf{k}) = \Sigma^{\text{im}}(E, \mathbf{k}) + \Sigma^{\text{el}}(E, \mathbf{k}) + \Sigma^{\text{ph}}(E, \mathbf{k}). \quad (1)$$

In ARPES, the self-energy  $\Sigma(E, \mathbf{k})$  is accessible from the spectral function  $A(E, \mathbf{k})$  [2] given a known dispersion relation  $\varepsilon(\mathbf{k})$  [2]. For the bare band dispersions fitted in this work, we use the following dispersion relation:

$$\varepsilon(\mathbf{k}) = E_F + \frac{\hbar^2}{2m_b} [(\mathbf{k} - \mathbf{k}_0)^2 - k_F^2], \quad (2)$$

where  $k_F$  is the Fermi wavevector,  $E_F$  is the Fermi level,  $m_b$  is the bare electron mass [3], and  $\mathbf{k}_0$  is a very small offset as the setup is not exactly at normal emission. The bare mass  $m_b \equiv (\nabla_{\mathbf{k}}^2 \varepsilon(\mathbf{k})/\hbar^2)^{-1}$  is the mass of the electrons upon placing them in a periodic potential, before considering the many-body effects captured by  $\Sigma(E, \mathbf{k})$  that turn them into dressed quasiparticles [4]. Along the direction of  $\hat{\mathbf{k}}_{[110]}$  of the band map of Fig. 4a of the main text,  $k_{[110]} = \mathbf{k} \cdot \hat{\mathbf{k}}_{[110]}$  and  $k_{0,[110]} = \mathbf{k}_0 \cdot \hat{\mathbf{k}}_{[110]}$ , where we used  $k_{0,[110]} = -0.0065 \text{ \AA}^{-1}$  to symmetrize the results displayed in Fig. 4 of the main text and Fig. SM7.

Along  $k_{[110]}$ , the spectral function [2] for a single band at an energy  $E_j$  can be written as:

$$A(E_j, k_{[110]}) = \frac{1}{\pi} \frac{-\Sigma''(E_j, k_{[110]})}{[E_j - \varepsilon(k_{[110]}) - \Sigma'(E_j, k_{[110]})]^2 + \Sigma''^2(E_j, k_{[110]})}, \quad (3)$$

where  $j$  is the energy index corresponding to the energy discretization of the band map. Unfortunately, the spectral intensity along  $k_{[110]}$  decays rapidly away from the MDC maximum, so that there is insufficient signal to determine the  $k_{[110]}$ -dependence of  $\Sigma(E_j, k_{[110]})$ . Instead of neglecting the momentum dependence, we seek a relation for an energy  $E_j$  and a corresponding momentum value  $k_{[110],j}$  that best represents the momentum dependence of the self-energy at  $E_j$ . In other words, we wish to establish the following parametrization:

$$\Sigma(E_j, k_{[110]}) \approx \Sigma(E_j, k_{[110],j}) = \Sigma(E_j(k_{[110],j})) = \Sigma(E_j). \quad (4)$$

We emphasize that the leftmost quantity in Eq. 4 is a 2D variable, while the three rightmost quantities are different notations for the corresponding 1D variable. The rightmost notation in Eq. (4) is applicable in our case because our MDC maxima move towards  $E_F$  monotonically with  $|k_{[110]} - k_{0,[110]}|$  and we consistently refer to the inner and outer left-hand and right-hand branches. Note that an equivalent parametrization can be obtained from the analysis of energy distribution curves for each  $k_{[110],j}$ . To arrive at Eq. 4, we argue that for a  $\Sigma(E_j, k_{[110],j})$  that does not change rapidly over  $k_{[110],j}$ , the momentum dependence at an energy  $E_j$  is best described by the momentum value  $k_{[110],j}$  corresponding to the peak in the MDC, which is given by:

$$E_j - \varepsilon(k_{[110],j}) - \Sigma'(E_j, k_{[110],j}) = 0. \quad (5)$$

The validity of the approximation of Eq. 4 is experimentally evaluated by the quality of an MDC fit: A strong momentum dependence of  $\Sigma(E_j, k_{[110]})$  should result in a poor MDC fit when using  $\Sigma(E_j)$ . After determining the self-energies and bare band parameters of Eq. 2, the momenta for the left-hand (−) and right-hand branches (+) can be obtained as:

$$k_{[110],j} = k_{0,[110]} \pm \left\{ k_F^2 + \frac{2m_b}{\hbar^2} [E_j - E_F - \Sigma'(E_j)] \right\}. \quad (6)$$

We link the electron momentum to the geometry of the ARPES experiment following the notation of Ref. [5], although we drop the  $k$ -label on the azimuthal angle  $\phi$  and the polar angle as  $\theta$ . We fix  $\phi = 45^\circ$  as well as the light polarization  $\boldsymbol{\epsilon} = e^{i\eta} \epsilon_x \hat{x}$  [5] for  $s$ -polarized light, where  $\epsilon_x$  is the  $x$ -component of  $\boldsymbol{\epsilon}$  and  $\eta$  is the light phase. For this value of  $\phi$ ,  $k_{[110]}$  is parametrized in terms of the polar angle  $\theta$  as  $k_{[110]} = \sqrt{2m_e E_{\text{kin}}/\hbar^2} \sin(\theta)$ , where  $E_{\text{kin}} = h\nu - E_{\text{bin}} - \Phi$

is the kinetic energy of the escaping photoelectron,  $m_e$  is the electron rest mass,  $E_{\text{bin}}$  is the electron binding energy, and  $\Phi = 4.33$  eV is the work function of the ARPES setup. For this  $\epsilon$  and the parametrization of  $k_{[110]}$  in terms of  $\theta$ , we can denote the spectral function as  $A(E, \theta)$  and the polarization term of the photoemission matrix element as  $M(E, \theta)$ . A description of these quantities in terms of  $\theta$  is needed to convolve with a constant resolution of  $\Delta\theta$ , after which we will switch back to a  $k_{[110]}$ -based notation. We assume that over the band maps of  $\mathcal{O}(100$  meV), the total photoemission matrix element is dominated by the polarization term  $M(E, \theta)$ . This assumption is motivated by observing that the  $E$ -dependence in the  $h\nu$  scan in Figs. 2a,b of the main text from the other orbital contributions changes on the scale of  $\mathcal{O}(1$  eV) and by the fact that we are very close to normal emission. Therefore, we treat the momentum conservation, out-of-plane component, and orbital matrix elements [5] as constant over this region.

To arrive at an expression for the photocurrent [2], we first multiply the spectral function  $A(E, \theta)$  with the modulus-squared orbital matrix element  $|M(E, \theta)|^2$  and the Fermi-Dirac distribution  $f(E)$ . Next, we convolve with Gaussian distributions for the energy resolution  $R$  and angular resolution  $Q$  and add a background term  $B(E)$ , yielding the photocurrent as:

$$I(E, \theta) = C_0 \iint dE' d\theta' [|M(E', \theta')|^2 f(E') A(E', \theta') R(E - E') Q(\theta - \theta') + B(E')], \quad (7)$$

where  $C_0$  is a fitting constant, and where we estimate the energy resolution to be  $\Delta E = 10.0$  meV from the Fermi-Dirac edge [6] and use an angular resolution of  $\Delta\theta = 0.2^\circ$  [7]. Note that  $f(E)$  and the kernel function  $K(E, \omega)$  defined in Eq. (15) are implicitly dependent on the temperature of  $T = 21.5$  K used in the experiment. Time integration over  $I(E, \theta)$  yields the photointensity, which we denote as  $P(E, \theta)$ .

Before performing the self-energy analysis, we estimate how the polarization matrix element varies over the band map of Fig. 4a of the main text. We will denote fitting the photocurrent using a specific photoemission matrix element as the matrix element correction (MEC). As the  $\theta$ -dependence of  $|M(E, \theta)|^2$  is usually much larger than the  $E$ -dependence of the polarization matrix element over a band map [5], we assume  $|M(E, \theta)|^2 = |M(\theta)|^2$ . To proceed, we integrate over the  $E$  to obtain the energy-integrated photointensity denoted as  $P(\theta)$ . The resulting  $P(\theta)$  can subsequently be compared with the sum rule [2]:

$$\int_{-\infty}^{\infty} dE A(E, \theta) = 1, \quad (8)$$

stating that for parabolic bands, every non-degenerate band adds one unit of spectral weight for  $|\theta| \lesssim \theta_F$ , where  $\theta_F = 2.25^\circ$  is the Fermi angle of the inner band. By comparing Eqs. (7) and (8), we infer that for  $|\theta| \lesssim \theta_F$ ,  $I(\theta)$  should be proportional to  $|M(\theta)|^2$ , aside from the convolution. To reproduce  $P(\theta)$  for  $|\theta| \lesssim \theta_F$ , we choose  $|M(\theta)|^2 = C_1 \sin^2(\theta)$  instead of an using no correction with  $|M(\theta)|^2 = C_2$ , where  $C_1$  and  $C_2$  are real constants. This functional form reproduces well the energy-integrated photoemission intensity  $P(\theta)$  simulated as  $P(\theta) = C_3 \sin^2(\theta) + C_4 B$  with real constants  $C_3$  and  $C_4$  as well as the energy-integrated  $B$ , as shown in Fig. SM7a.

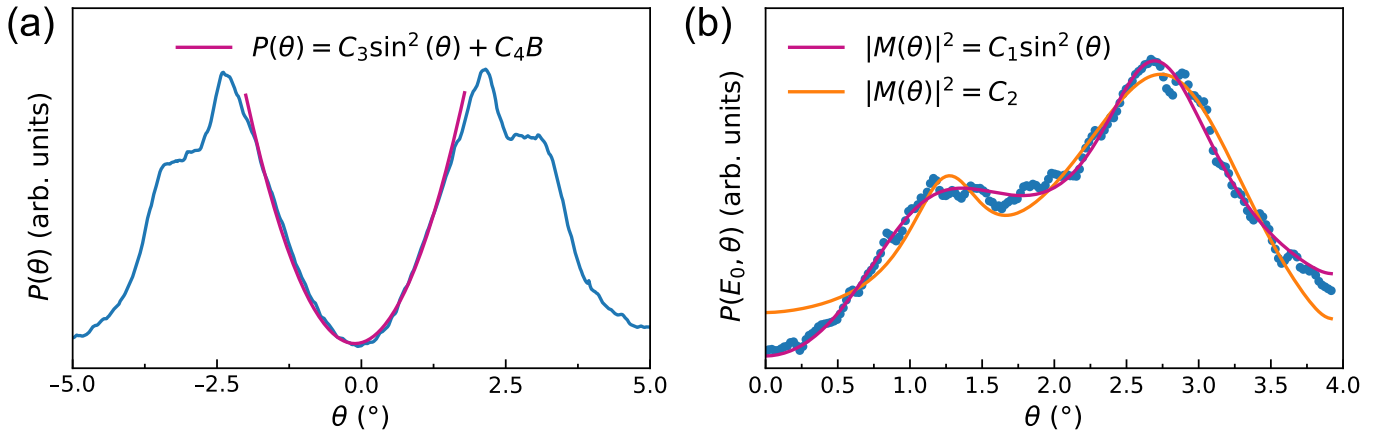

FIG. SM7. **Motivation for the choice of matrix elements.** (a) Energy-integrated photoemission intensity  $P(\theta)$  (blue) from the  $\text{TiO}_2$ -terminated band map compared to the simulated  $P(\theta) = C_3 \sin^2(\theta) + C_4 B$  (magenta), where  $C_3$  and  $C_4$  are real constants. (b) Comparison of momentum distribution curve fits  $P(E_0, \theta)$  at an electron energy of  $E_0 = E_F - 100$  meV for matrix elements  $|M(\theta)|^2 = C_1 \sin^2(\theta)$  versus  $|M(\theta)|^2 = C_2$ , where  $C_1$  and  $C_2$  are real constants.

The obtained element provides better agreement compared to a constant  $|M(\theta)|^2 = C_2$  upon fitting the MDC branches, as shown in Fig. SM7b at a representative electron energy  $E_0 = E_F - 100$  meV. The matrix elements

$|M(\theta)|^2 = C_1 \sin^2(\theta)$  are fitted with respect to  $\theta_0 = -0.10^\circ$ , corresponding to  $k_{0,[110]}$  at  $E_{\text{bin}} = 0$ . Lastly, we remark that the  $|M(\theta)|^2 = C_1 \sin^2(\theta)$  dependence is identical to the  $\theta$ -dependence of a gas-based  $d_{xy} \rightarrow p$  transition for our  $s$ -polarization  $\epsilon \parallel \hat{x}$  [8]. This suggests that from a three-step model perspective [2] at  $h\nu = 47$  eV, the energy of the escaping photoelectron is such that it can transition to an available  $p$ -orbital, but there is no notable contribution from the transition towards the  $f$ -orbital. However, a full description of the photoemission matrix element would require a theory adapted to periodic systems, such as the recent scattered-wave approximation [9]. Nonetheless, our heuristically obtained  $|M(\theta)|^2$  improves the quality of the self-energy extraction and is therefore used as the MEC in this work.

Having performed the convolution in Eq. 7, we switch back to a notation in terms of the projected wavevector  $k_{[110]} = \sqrt{2m_e E_{\text{kin}}/\hbar^2} \sin(\theta)$  that describes the electron wavevectors. Having selected  $|M(\theta)|^2$ , we simultaneously fit the dispersion relations  $\varepsilon(\mathbf{k})$  and self-energies  $\Sigma(E)$  for the left-hand and right-hand sides of the band map. This procedure generates the MDC maxima shown in Fig. 4a of the main text alongside two parabolas for the inner and outer bands with  $m_b = 0.6 m_e$  determined from inspection, which will be optimized Section SM7. The Fermi level  $E_F$  is obtained for all of the electron branches from the Fermi-Dirac edge [6]. We then obtain the set of two Fermi wavevectors  $\{k_F\}$  and parabolic minimum  $k_{0,[110]}$  by setting  $\Sigma'(E_F) = 0$  for the left- and right-hand side parabolas.

Using the determined  $k_F = 0.21 \text{ \AA}^{-1}$  and initial effective mass  $m_b = 0.6 m_e$ , we extract the real and minus imaginary parts of the self-energies and report them with 95% confidence intervals in Figs. SM8a and SM8b, respectively.

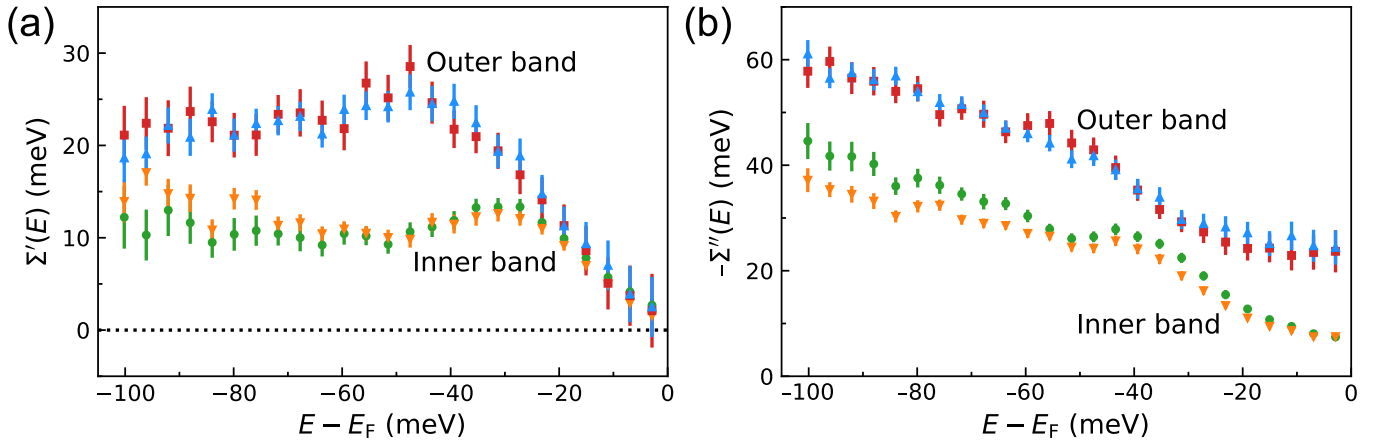

FIG. SM8. **Detailed self-energies for the  $d_{xy}$  bands of the  $\text{TiO}_2$ -terminated surface.** (a) Real  $\Sigma'(E)$  and (b) minus imaginary  $-\Sigma''(E)$  parts of the self-energy for the outer left-hand (red squares) and right-hand (blue upward triangles) branches, as well as for the inner left-hand (orange circles) and right-hand (green downward triangles) branches of the intense  $d_{xy}$  bands for the  $\text{TiO}_2$ -terminated surface at  $h\nu = 47$  eV. Vertical bars denote 95% confidence intervals obtained from the MDC fitting.

The self-energies show a strong similarity for different branches of individual parabolas, while displaying more dissimilarity between the different parabolas. The dissimilarity between the bands likely originates from the different electron momenta of the photoemission kinks, and does not preclude a specific origin of the lifted degeneracy of the  $d_{xy}$ -derived bands. Furthermore, the self-energies for the outer bands are comparable in magnitude to those reported in a previous study [10], where slight differences may arise from our use of a MEC. For the self-energies in SM8, the faint inner bands were not fitted because of the difficulty in determining in which binding energy range they should be accounted for. This choice may lead to a slight bias in the self-energies, particularly for the inner bands at low binding energies.

Finally, the real and minus imaginary parts of the inner band self-energies show a dip at  $E \approx 50$  meV. This dip likely originates from the intersection of the inner band with one of the bulk-derived bands [10]. The presence of the bulk-derived band may cause the MDC width to be a weighted average of the widths of the bulk-derived and  $d_{xy}$ -derived bands, either due to complete band hybridization or because part of the photointensity comes from the bulk-derived band separately. By comparing cut #1 from Fig. 1e of the main text with the bulk-derived bands visible in Fig. 2c of the main text, we infer that the bulk-derived bands intersect with the inner  $d_{xy}$ -derived bands on the band map, but not with the outer ones. Incorporating such band intersections is beyond the scope of this study. Therefore, in Section SM7 we only extract  $\alpha^2 F(\omega)$  from the outer  $d_{xy}$  band, which does not display such a dip.

### SM6. BARE BAND PARAMETERS

In this section, we report the bare band parameters for the  $h\nu \in \{47 \text{ eV}, 85 \text{ eV}\}$  TiO<sub>2</sub>- and SrO-terminated band maps. Although the different SrTiO<sub>3</sub> bands have been characterized previously [11], we report the quantities specifically for the TiO<sub>2</sub> and SrO-terminated surfaces. For the TiO<sub>2</sub>-terminated surface at  $h\nu = 85 \text{ eV}$ , we identify the  $d_{yz}$ -derived band along the  $k_x$ -axis, in addition to the two non-degenerate  $d_{xy}$ -derived bands that are also observed at  $h\nu = 47 \text{ eV}$ . For the SrO termination, we identify a single  $d_{xy}$ -derived band at both photon energies, in addition to the  $d_{xz}$ - and  $d_{yz}$ -derived bands at  $h\nu = 85 \text{ eV}$ .

First, we perform a simultaneous fitting for the MDCs of each band map, which yields  $\varepsilon(\mathbf{k})$  and  $\Sigma'(E)$  upon determining  $m_b$  by visual inspection. The photoemission matrix elements of the  $d_{xz}$ -derived and  $d_{yz}$ -derived bands do not display notable momentum dependence at  $h\nu = 85 \text{ eV}$  (see Figs. 2c,d). Consequently, no MEC was applied for these bulk-derived bands on either termination. For the  $d_{xy}$ -derived bands, we find that applying the MEC discussed in Section SM5 leads to a better fitting for both surface terminations. This suggests that even for the SrO-terminated surface, the 2DEL exists in the Ti  $d_{xy}$ -orbitals provided by one or more layers of TiO<sub>2</sub>. The observation of Ti-derived states at both surface terminations is also in agreement with the energies of the resonance enhancement being equal at both terminations (Figs. 2a and 2b of the main text). For the  $h\nu = 85 \text{ eV}$  band maps, the RMMESH code [12] was employed to remove Fourier components of the detector mesh. Given the low signal-to-noise ratio of the innermost ( $d_{xz}$ -derived) band of the SrO-terminated surface at  $h\nu = 85 \text{ eV}$ , the MDC peak width was limited to a maximum of  $0.01 \text{ \AA}^{-1}$  to prevent the peak from smearing out over the noise.

TABLE SM1. Bare band parameters for the  $d$ -derived bands of the TiO<sub>2</sub>- and SrO-terminated surfaces at  $h\nu \in \{47 \text{ eV}, 85 \text{ eV}\}$ .

| TiO <sub>2</sub> termination       |                    |                         |                                      |             |                              |
|------------------------------------|--------------------|-------------------------|--------------------------------------|-------------|------------------------------|
|                                    | Band               | $k_F (\text{\AA}^{-1})$ | $n_{2D}/g (10^{12} \text{ cm}^{-2})$ | $m_b (m_e)$ | $E_{\text{bot}} (\text{eV})$ |
| 47 eV $d_{xy}$                     | Intense outer      | 0.210                   | 35.1                                 | 0.6         | 0.28                         |
|                                    | Intense inner      | 0.140                   | 15.6                                 | 0.6         | 0.12                         |
|                                    | Faint outer        | 0.10                    | 8.0                                  | —           | —                            |
|                                    | Faint inner        | 0.076                   | 4.6                                  | —           | —                            |
| 85 eV $d_{xy}$                     | Intense outer      | 0.22                    | 39                                   | 0.6         | 0.31                         |
|                                    | Intense inner      | 0.15                    | 18                                   | 0.6         | 0.14                         |
| $n_{3D} (10^{20} \text{ cm}^{-3})$ |                    |                         |                                      |             |                              |
| 85 eV $d_{yz}$                     | Single             | 0.41                    | 1.1                                  | 10          | 0.06                         |
| SrO termination                    |                    |                         |                                      |             |                              |
| $n_{2D} (10^{12} \text{ cm}^{-2})$ |                    |                         |                                      |             |                              |
| 47 eV $d_{xy}$                     | Single             | 0.17                    | 46                                   | 0.6         | 0.18                         |
| 85 eV $d_{xy}$                     | Single             | 0.18                    | 52                                   | 0.6         | 0.23                         |
| $n_{3D} (10^{20} \text{ cm}^{-3})$ |                    |                         |                                      |             |                              |
| 85 eV $d_{xz/yz}$                  | Outer ( $d_{yz}$ ) | 0.40                    | 1.1                                  | 10          | 0.06                         |
|                                    | Inner ( $d_{xz}$ ) | 0.09                    | 1.1                                  | 0.5         | 0.06                         |

Next, we determine the Fermi wavevectors  $k_F$  by assuming  $\Sigma'(E = E_F) = 0$  as reported in Tab. SM1. The difference in precision for the quantities is reported with significant figures and is primarily due to different measurement integration times. The bands and the fitted MDC maxima are shown on top of the band maps in Fig. SM9, where we used offsets of (a)  $k_{0,[100]} = -0.54 \text{ \AA}^{-1}$ , (b)  $k_{0,[100]} = -0.057 \text{ \AA}^{-1}$ , and (c)  $k_{0,[110]} = -0.018 \text{ \AA}^{-1}$ , respectively. From visual inspection, we determine  $m_b = 0.6 m_e$  for the  $d_{xy}$ -derived bands,  $m_b = 10 m_e$  along the  $k_x$ -axis for the  $d_{yz}$ -derived bands, and  $m_b = 0.5 m_e$  along the  $k_x$ -axis of the  $d_{xz}$ -derived band, observed only for the SrO termination at  $h\nu = 85 \text{ eV}$ . Subsequently, we calculate the band bottoms  $E_{\text{bot}} = \hbar^2 k_F^2 / (2m_b)$ . We then calculate the charge densities for the bands based on the Luttinger volumes. Because the spin splitting of the light bands is still under debate [13, 14], we report  $n_{2D}/g = k_F^2 / (4\pi)$  for the TiO<sub>2</sub> main bands as well as their replicas, where  $g$  is the degeneracy for a spin-polarized ( $g = 1$ ) or spin-degenerate ( $g = 2$ ) band. For the  $d_{xy}$  band of the SrO-terminated surface, it was not possible to decisively determine the number of peaks (see Section SM3). Therefore, we take a conservative approach and fit only a single band at both photon energies, while reporting the spin-degenerate  $n_{2D} = k_F^2 / (2\pi)$ .

For the bulk-derived bands, we assume the shapes of prolate spheroids, such that the carrier density is  $n_{3D} = k_{F,a}^2 k_{F,c} / (3\pi^2)$  (where  $k_{F,a}$  and  $k_{F,c}$  are the respective short and long axes of the spheroid) found for bulk first-principles

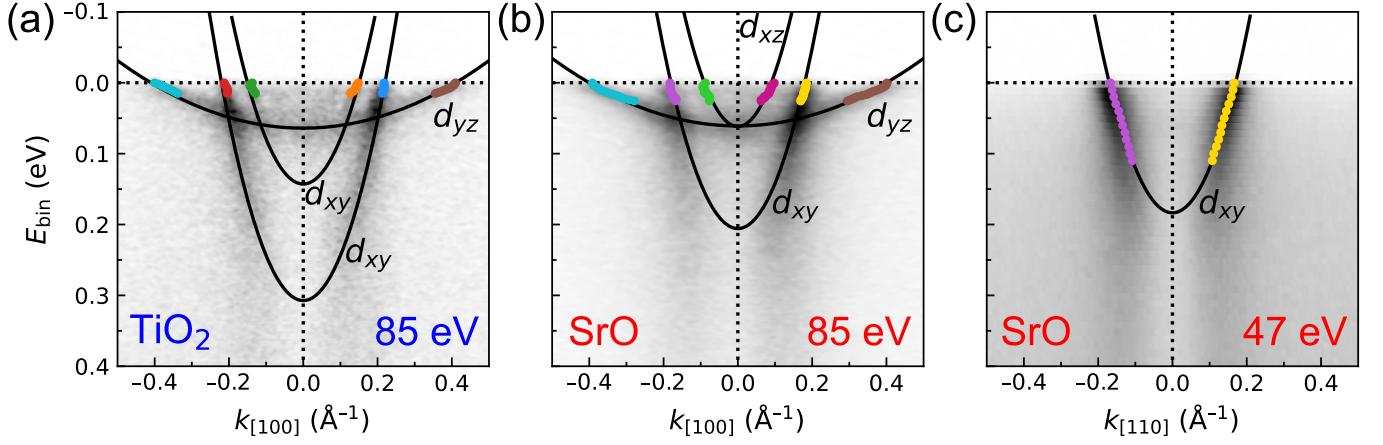

FIG. SM9. Band maps, bare bands (continuous lines), and MDC maxima (colored dots) for (a) the  $\text{TiO}_2$ -terminated surface at photon energy  $h\nu = 85$  eV and for the SrO-terminated surface at (b)  $h\nu = 85$  eV and (c)  $h\nu = 47$  eV. Identical color coding of the MDC maxima between the band maps is used to emphasize similar band origins at different photon energies. Parameters for the bands are found in Tab. SM1. The  $h\nu = 85$  eV band maps were taken along  $k_{[100]}$  (cut # 2), whereas the  $h\nu = 47$  eV band map was taken along  $k_{[110]}$  (cut # 1).

calculations [15]. Notably, our data does not contain any  $k_z$ -dispersion and therefore precludes quantification of a previously observed stretching along  $k_z$  that leads to an ellipsoidal shape [11]. For determining  $n_{3D}$  of the SrO-terminated surface at  $h\nu = 85$  eV, we only have  $k_{F,c}$  for the  $d_{yz}$ -derived spheroid and  $k_{F,a}$  for the  $d_{xz}$ -derived spheroid. Therefore, we assume that the  $d_{xz}$  and  $d_{yz}$  bands on this surface have the same  $k_{F,a}$  and  $k_{F,c}$  as motivated by Figs. 2c,d. For determining  $n_{3D}$  of the  $d_{yz}$  band of the  $\text{TiO}_2$ -terminated surface, we assume that its  $k_{F,a}$  is equal to the  $k_{F,a}$  of the  $d_{xz}$  band observed on the SrO-terminated surface.

### SM7. ELIASHBERG SPECTRAL FUNCTION ANALYSIS

In this section, we detail the extraction of the Eliashberg spectral function  $\alpha^2 F(\omega)$  of the left-hand and right-hand outer branches of the  $\text{TiO}_2$ -terminated surface at  $h\nu = 47$  eV using a Bayesian inference procedure [16], which allows for optimizing per branch the effective mass  $m_b$ , the Fermi wavevector  $k_F$ , the static imaginary part of the impurity self-energy  $\Sigma^{\text{im}''}$ , the electron-electron scattering magnitude  $g^{\text{el-el}}$ , and the default model plateau height  $m_0$ . Additionally, we perform a quantitative comparison of the left-hand and right-hand Eliashberg functions, which can be performed because the data surrounds the surface high-symmetry point  $\bar{\Gamma}_{00}$ , resulting in a small asymmetry of the photoemission matrix elements. Close to  $\bar{\Gamma}_{00}$ , the photointensity is strongly suppressed due to the photoemission matrix elements. However, we have corrected for this effect with the MEC described in Section SM5. Furthermore, we disregard the extracted self-energies in an interval  $\Delta E = 10$  meV near  $E = E_F$  as these values are most heavily affected by the energy convolution.

The most likely Eliashberg function  $\widehat{\alpha^2 F}(\omega)$  is obtained using Bryan's implementation [17] of the maximum entropy method (MEM) [18]:

$$\widehat{\alpha^2 F}(\omega) = \arg \max_{\alpha^2 F(\omega)} L_D + aS, \quad (9)$$

where  $a$  is a regularization parameter or Lagrange multiplier that we obtain from marginalization [17],  $L_D$  is the data-dependent part of the log-likelihood [19], and where we include prior knowledge on the Eliashberg function through the information entropy  $S$ . We discretize the interval of  $\alpha$  from  $\alpha_{\min} = 0.5$  to  $\alpha_{\max} = 10$  (left-hand self-energies) and  $\alpha_{\max} = 15$  (right-hand self-energies) to ensure that the entire probability curve of  $\alpha$  is contained in this interval. Strictly speaking, the total log-likelihood  $L$  contains an additional sum over the standard deviations of the data [19]. However, this term is typically neglected in the MEM community [17, 18]. For simplicity, we denote the solution from Eq. (9) as  $\alpha^2 F(\omega)$  throughout the rest of this work. In Eq. (9),  $L_D$  can be expressed in terms of  $N_J$  values at energies  $E_j$  for the real self-energy data  $\tilde{\Sigma}'(E_j)$ , its corresponding fit  $\Sigma'(E_j)$ , squared standard deviations  $\sigma_j'^2$ , and the counterparts for the imaginary self-energies ( $\tilde{\Sigma}''(E_j)$ ,  $\Sigma''(E_j)$ ,  $\sigma_j''^2$ ):

$$L_D = - \sum_{j=1}^{N_J} \left\{ \frac{[\tilde{\Sigma}'(E_j) - \Sigma'(E_j)]^2}{2\sigma_j'^2} + \frac{[\tilde{\Sigma}''(E_j) - \Sigma''(E_j)]^2}{2\sigma_j''^2} \right\}. \quad (10)$$

Throughout the rest of this work, we refer to the experimental data without the tildes for simplicity. We use the following expression for the Shannon-Jaynes information entropy [18] in Eq. (9):

$$S = \sum_{l=1}^{N_L} \left\{ \alpha^2 F(\omega_l) - m(\omega_l) - \alpha^2 F(\omega_l) \ln \left[ \frac{\alpha^2 F(\omega_l)}{m(\omega_l)} \right] \right\}, \quad (11)$$

where the phonon energy spectrum has been discretized over  $N_L = 500$  evenly spaced image points for  $\omega_l \in [1 \text{ meV}, 120 \text{ meV}]$ . In Eq. (11),  $m(\omega)$  is a default model [18] used to restrict the spectral function in the relevant energy range:

$$\frac{m(\omega)}{m_0} = \begin{cases} 2 \left( \frac{\omega}{\omega_I} \right)^2 & 0 \leq \omega < \frac{\omega_I}{2} \\ 1 - 2 \left( \frac{\omega}{\omega_I} - 1 \right)^2 & \frac{\omega_I}{2} \leq \omega < \omega_I \\ 1 & \omega_I \leq \omega < \omega_M \\ 1 - 2 \left( \frac{\omega - \omega_M}{\omega_I} \right)^2 & \omega_M \leq \omega < \omega_M + \frac{\omega_I}{2} \\ 2 \left( \frac{\omega - \omega_M}{\omega_I} - 1 \right)^2 & \omega_M + \frac{\omega_I}{2} \leq \omega < \omega_M + \omega_I, \end{cases} \quad (12)$$

where  $m_0$  is the plateau height,  $\omega_I = 20$  meV is an intermediate energy based on the onset of an intermediate EPC strength [20], and  $\omega_M = 100$  meV corresponds to the maximum phonon energy.

To minimize the quantity in Eq. (10), we need a description for the total self-energy  $\Sigma(E)$  from Eq. (1). For the imaginary part of the electron-electron self-energy  $\Sigma^{\text{el}''}(E)$ , we use the expression from Ref. [21] for  $T \rightarrow 0$  and  $E < E_F$ :

$$\Sigma^{\text{el}''}(E) = -g^{\text{el-el}} \frac{E_{\text{bot}}}{8\pi} \left( \frac{E}{E_{\text{bot}}} \right)^2 \left[ 2 \ln \left( -\frac{E_{\text{bot}}}{E} \right) + \ln(8) + 1 \right], \quad (13)$$

where  $g^{\text{el-el}}$  is the electron-electron scattering magnitude, denoted as  $w^{f,b}$  in Ref. [21]. The real part  $\Sigma^{\text{el}}$  is a small and nearly static contribution [21] that we assume to be 0. For the impurity self-energy, we consider a static imaginary term  $\Sigma^{\text{im}}(E) \rightarrow i\Sigma^{\text{im}''}$  [22]. We assume that  $\Sigma^{\text{ph}}(E)$  is dominated by the Fan-Migdal self-energy [23], such that we disregard the momentum dependence of Debye-Waller self-energy [23] over the range of the photomission kink, and we also disregard the self-energy diagrams that are of higher order in the scattering. Subsequently,  $\alpha^2 F(\omega)$  is obtained from inverting the following integral [24]:

$$\Sigma^{\text{ph}}(E) = \int_0^\infty d\omega \alpha^2 F(\omega) K(E, \omega), \quad (14)$$

where we use the following finite-temperature expression for the bosonic kernel [25]:

$$K(E, \omega) = \int_{-\infty}^\infty d\nu \left[ \frac{f(-\nu) + n(\omega)}{E - \omega - \nu + i\eta} + \frac{f(\nu) + n(\omega)}{E + \omega - \nu + i\eta} \right], \quad (15)$$

where  $\eta$  is an infinitesimal value from the analytic continuation [26] that we set numerically to  $10^{-5}$  meV.

We reduce the integration range of Eq. (15) by assuming that scattering only occurs from the band bottom  $E_{\text{bot}} - E_F$  to an equivalent energy  $E_{\text{bot}} + E_F$ :

$$K(E, \omega) = \int_{E_F - E_{\text{bot}}}^{E_F + E_{\text{bot}}} d\nu \left[ \frac{f(-\nu) + n(\omega)}{E - \omega - \nu + i\eta} + \frac{f(\nu) + n(\omega)}{E + \omega - \nu + i\eta} \right]. \quad (16)$$

The expression for  $K(E, \omega)$  in Eq. 16 can then be integrated to give the following analytic expression [24]:

$$K(E, \omega) = -i\pi + \psi \left( \frac{1}{2} - i \frac{E - E_F - \omega + i\eta}{2\pi k_B T} \right) - \psi \left( \frac{1}{2} - i \frac{E - E_F + \omega + i\eta}{2\pi k_B T} \right) + \ln \left( \frac{E - E_F + \omega + E_{\text{bot}} + i\eta}{E - E_F + \omega + E_{\text{bot}} + i\eta} \right) \\ + n(\omega) \left[ \ln \left( \frac{E - E_F - \omega + E_{\text{bot}} + i\eta}{E - E_F - \omega - E_{\text{bot}} + i\eta} \right) + \ln \left( \frac{E - E_F + \omega + E_{\text{bot}} + i\eta}{E - E_F + \omega - E_{\text{bot}} + i\eta} \right) \right], \quad (17)$$

where  $\psi(x)$  is the digamma function.

From the optimization step, we obtain the imaginary contributions of  $-\Sigma^{\text{im}''} = 24.2$  meV and  $-\Sigma^{\text{im}''} = 20.7$  meV for the respective right-hand and left-hand outer branches. By contrast, the offset of the inner bands  $-\Sigma^{\text{im}''} \approx 7$  meV is smaller, which suggests that the electrons of the inner band experience the impurities differently. From the optimization, we also find that the  $g^{\text{el-el}}$  in Eq. (13) are effectively 0 for both branches. Consequently, the electron contribution of  $\Sigma^{\text{el}}(E)$  is found to be negligible in our system. We remark that  $\Sigma^{\text{el}}(E)$  primarily affects the MDC width, which might change when incorporating the energy resolution in the MDC fitting. Therefore, the theoretically predicted  $-\Sigma^{\text{el}''}$  of  $\mathcal{O}(1)$  meV for our system at  $T \ll T_F = E_F/k_B$  [21] might be too small to resolve while neglecting the energy convolution. Further research into the energy resolution effects will be necessary to uncover the magnitude of  $-\Sigma^{\text{el}''}$  in our system.

The self-energies for the left-hand outer parabola are shown in Fig. SM10a for an optimized  $m_b = 0.62 m_e$  and  $k_F = 0.2109 \text{ \AA}^{-1}$ . Figure SM10b shows the left-hand  $\alpha^2 F(\omega)$  together with its model function  $m(\omega)$  and its 95% confidence interval. This confidence interval was obtained by propagating the self-energy uncertainties [16]. The spectral features at  $\omega = 54$  meV,  $\omega = 69$  meV, and  $\omega = 88$  meV in the left-hand  $\alpha^2 F(\omega)$  may be related to the respective  $\text{LO}_3$ ,  $\text{TO}_4$ , and  $\text{LO}_4$  peaks from Ref. [27]. However, these peaks might also contain contributions from surface phonons found at similar energies in first-principles calculations [28] for the left-hand and right-hand Eliashberg functions. The  $\text{LO}_3$  mode now only appears as a shoulder because the outlier in  $\Sigma'(E)$  at  $E - E_F = -48$  meV induces a pronounced peak in  $\alpha^2 F(\omega)$  at  $\omega = 48$  meV. The left-hand default model  $m(\omega)$  was found to have an optimized plateau height of  $m_0 = 0.130$ , whereas the right-hand plateau height is  $m_0 = 0.129$ . We calculate the EPC parameter  $\lambda = -\partial \Sigma'(E)/\partial E|_{E=E_F}$  as the slope of the fit of  $\Sigma'(E)$ , represented by the continuous red line in Fig. SM10a. From the left-hand  $\Sigma'(E)$  reconstructed from  $\alpha^2 F(\omega)$ , we obtain  $\lambda = 0.68$ , yielding a quasiparticle effective mass of  $m^* = Z^{-1}m_b = 1.03 m_e$ , where  $Z = (1 + \lambda)^{-1} = 0.59$  is the quasiparticle residue [3] for the left-hand side. For the right-hand branch presented in Fig. 4b, we have optimized  $m_b = 0.59 m_e$  and  $k_F = 0.2096 \text{ \AA}^{-1}$ , and additionally we obtain  $\lambda = 0.63$ , which yields  $Z = 0.61$  and  $m^* = 0.96 m_e$ . These EPC quantities from the two branches are in good internal agreement, and the effective masses are in good agreement with  $m_b = 0.6 m_e$  obtained from visual inspection.

Lastly, we quantify the agreement between the left-hand outer Eliashberg function denoted explicitly as  $\alpha^2 F_L(\omega)$  and the right-hand outer Eliashberg function  $\alpha^2 F_R(\omega)$  by calculating the difference function  $\Delta \alpha^2 F(\omega) \equiv \alpha^2 F_L(\omega) - \alpha^2 F_R(\omega)$ . The 95% confidence interval of  $\Delta \alpha^2 F(\omega)$  is obtained from the uncertainties of the respective  $\alpha^2 F_L(\omega)$  and  $\alpha^2 F_R(\omega)$ . We assume that the covariances  $\sigma_{\text{LR}} = 0$  for all energies  $\omega_j$  as the left-hand and right-hand branches have

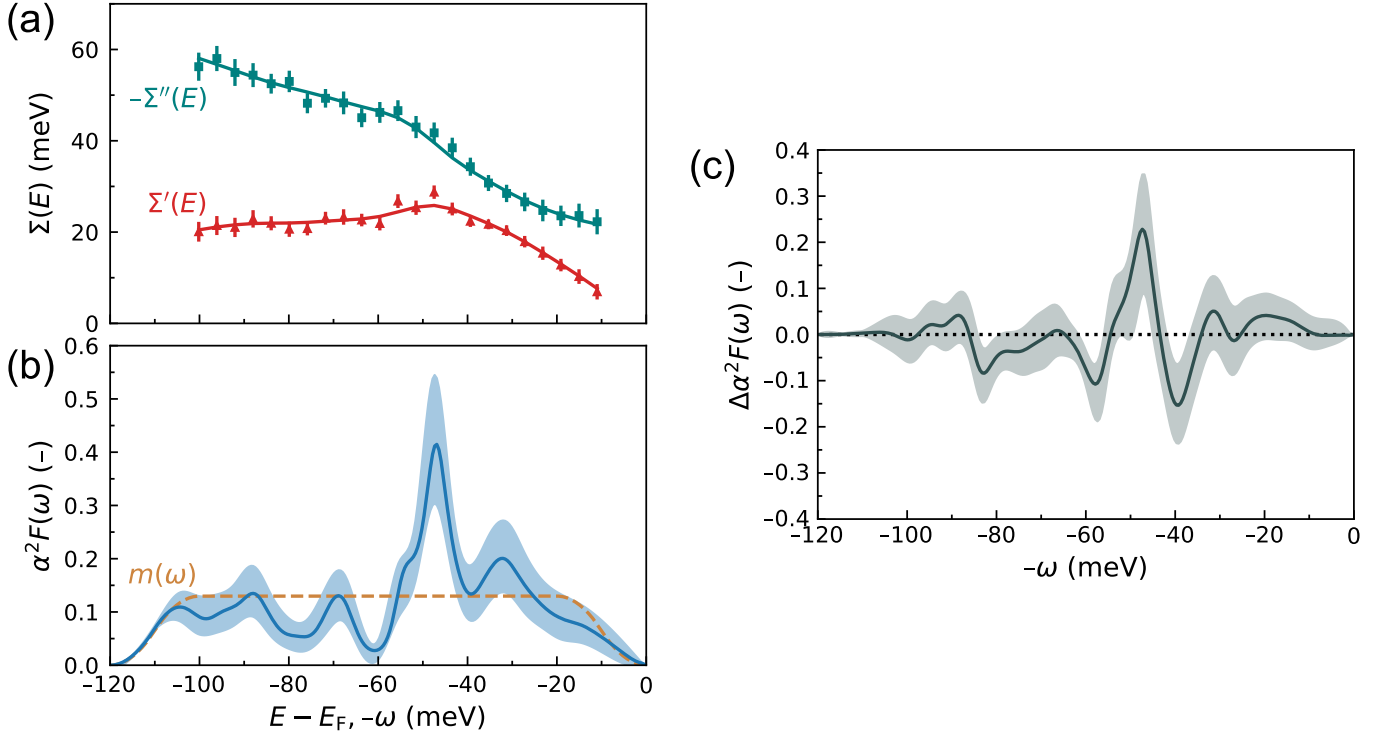

FIG. SM10. **Extraction of the left-hand Eliashberg function and comparison with the right-hand Eliashberg function presented in Fig. 4 from the main text.** (a) The self-energy components of the outer left-hand branch for  $m_b = 0.62 m_e$ . (b) The left-hand spectral function  $\alpha^2 F(\omega)$  with the optimized model function  $m(\omega)$ . The continuous line in b) is generated from the maximum entropy method using the self-energy data from a), while the shaded area is the 95% confidence interval. (c) The difference between the left-hand and right-hand Eliashberg functions  $\Delta\alpha^2 F(\omega)$  with its 95% confidence interval. The Eliashberg functions are in agreement for 83% of the values on the total energy interval.

been fitted separately. Therefore, if  $\alpha^2 F_L(\omega)$  and  $\alpha^2 F_R(\omega)$  are supposed to be identical, the confidence interval of  $\Delta\alpha^2 F(\omega_j)$  should include 0 for 95% of the energies. Figure SM10c shows  $\Delta\alpha^2 F(\omega)$  with its 95% confidence interval and gives an agreement for only 77% of the energy interval between  $\alpha^2 F_L(\omega)$  and  $\alpha^2 F_R(\omega)$ , which is still quite far below 95%. Further research will be needed to determine if there is a source of systematic uncertainty or if there is a broken radial symmetry reflected in two different Eliashberg functions.

### SM8. SPLITTING OF THE $d_{xy}$ BANDS ON THE TiO<sub>2</sub> TERMINATION

In this section, we evaluate the likelihood of a  $\Delta E$ -based splitting versus a  $\Delta k$ -based splitting for the  $d_{xy}$  bands at the TiO<sub>2</sub>-terminated surface of SrTiO<sub>3</sub> obtained at  $h\nu = 47$  eV. Although our measurements are not spin-resolved, we will subsequently refer to the  $\Delta E$ -based splitting as Zeeman-type [29] and to the  $\Delta k$ -based splitting as a Rashba-Dresselhaus-type (RD).

The splitting of these bands has been discussed previously [13, 14]. However, here we perform an analysis based on the extracted self-energies, relying on the fact that the real and imaginary parts are related via the Kramers-Kronig relations [30, 31]. Consequently, the Hilbert transform of the set of the imaginary data  $\mathcal{H}(\{\Sigma''(E_j)\})$  resemble the real data  $\Sigma'(E_j)$  for the correct choice of bare band parameters, a procedure known as “finding the bare band” [31] or “Kramers-Kronig bare-band fitting” (KKBF) [30], which has been applied to self-consistently obtain  $\Sigma'(E)$  and  $\Sigma''(E)$ , along with the dispersion relation. Therefore, we obtain the self-energies for the two types of bare band splittings, followed by comparing  $\mathcal{H}(\{\Sigma''(E_j)\})$  with  $\Sigma'(E_j)$  for both splittings, where  $\mathcal{H}(\{\Sigma''(E_j)\})$  is shorthand for the result at an energy  $E_j$  for the Hilbert transforming the available  $\{\Sigma''(E_j)\}$ . In both cases, we calculate the following error criterion:

$$C = \sqrt{\frac{1}{N_J} \sum_{j=1}^{N_J} \frac{[\Sigma'(E_j) - \mathcal{H}(\{\Sigma''(E_j)\})]^2}{\sigma_j'^2}}, \quad (18)$$

which shows how much by how many standard deviations the data points deviate from the model on average. For both splitting types, we simultaneously use the data from the two rightmost branches, to decide if a single bare band mass  $m_b$  can yield agreement between  $\Sigma'(E)$  and  $\mathcal{H}(\{\Sigma''(E_j)\})$  for both bands simultaneously. We perform this error minimization with 3 fitting parameters discussed below per dispersion relation.

An energy splitting  $\Delta E$  leads to two superimposed bands described by Eq. (2). A splitting of the band minima by momentum  $2\Delta k$  leads to two crossing bands, which are described by the following dispersion relation:

$$\varepsilon(k_{[110]}) = E_F + \frac{\hbar^2}{2m_b} [(k_{[110]} - k_{0,[110]} \pm \Delta k)^2 - k_F^2]. \quad (19)$$

The Rashba parameter  $\alpha_R$  can subsequently be calculated as  $\alpha_R = \hbar^2 \Delta k / m_b$ . We use the formulation in Eq. (19) rather than the more common expression [32] explicit in  $\alpha_R$  because the MDC analysis of our code [16] requires the dispersion relation to be a power function in  $k_{[110]} - k_{0,[110]}$ . For the RD-type splitting, the three automatic fitting parameters are the single bare band mass  $m_b$ ,  $\Delta k$ , and  $k_F$ . Notably,  $\Delta k$  needs to be fixed during the MDC fitting step, such that a range of  $\Delta k$  is tested to find its optimal value. For the Zeeman-type splitting, the three fitting parameters are the Fermi wavevectors for the respective inner and outer bands, and a single  $m_b$ . Although Zeeman-split bands can have two different effective masses, we use a single  $m_b$  such that both dispersion relations have three automatic optimization parameters for a fair comparison.

To perform the Hilbert transform, we use the `SCIPY.FFTPACK.HILBERT` function from the SciPy library [33]. Since we have a finite set of noisy data,  $\mathcal{H}(\{\Sigma''(E_j)\})$  will not perfectly reconstruct  $\Sigma'(E_j)$ , with larger deviations expected near the energy end points of the data sets. The deviations near  $E = E_F$  can be circumvented because  $-\Sigma''(E)$  is an even function with respect to  $E_F$ . Thus, before performing the Hilbert transform, we map the imaginary parts from the set of  $\{E_j\}$  below  $E_F$  towards the values  $\{-E_j\}$  above  $E_F$  by assuming that  $-\Sigma''(E_j) = -\Sigma''(-E_j)$ . Subsequently, we determine  $\mathcal{H}(\{\Sigma''(E_j)\})$  over the energy range symmetric around  $E_F$  and compare the results for the energies  $\{E_j\}$  below  $E_F$  to  $\Sigma'(E_j)$ .

We start out by obtaining initial guesses for the two  $k_F$  for the Zeeman-type splitting, and the  $k_F$  and  $\Delta k$  of the RD-type splitting, by assuming  $\Sigma'(E = E_F) = 0$  from the MDC maxima. We note that the MDC maxima obtained using Eq. (19) instead of Eq. (2) are slightly different. From this assessment, we find  $k_F = 0.21 \text{ \AA}^{-1}$  and  $k_F = 0.14 \text{ \AA}^{-1}$  for the Zeeman-type bands as listed in Table SM1, and  $k_F = 0.175 \text{ \AA}^{-1}$  as well as  $\Delta k = 0.035 \text{ \AA}^{-1}$  for the RD-type bands. Next, we obtain initial guesses for the effective masses of the inner and outer Zeeman-type bands and the left-hand and right-hand RD-type bands from visual inspection, finding  $m_b = 0.6 m_e$  for the Zeeman-type bands as listed in Table SM1, and an identical  $m_b = 0.6 m_e$  for the RD-type band. The MDC maxima and initial guesses for the bare bands are displayed in Fig. SM11a-b. It can be seen in Fig. SM11b that it is difficult to assign a single  $m_b$  that yields a typical photoemission kink simultaneously for both RD-split bands, where the MDC maxima are expected to decay towards the bare band at  $E_{\text{bin}}$  past the phonon bandwidth [23].

Starting from our initial guesses, we perform the optimization for the three parameters for both splitting types. The Zeeman-type splitting optimization yields  $m_b = 0.64 m_e$ ,  $k_F = 0.142 \text{ \AA}^{-1}$  and  $k_F = 0.209 \text{ \AA}^{-1}$  for the respective inner and outer branch. It can be seen in Fig. SM11c that the  $\mathcal{H}(\{\Sigma''(E_j)\})$  reconstruct the  $\Sigma'(E_j)$  well simultaneously

for the inner and outer right-hand branch Zeeman-type splitting. For the RD-type splitting, the optimization yields  $m_b = 0.73 m_e$ ,  $k_F = 0.179 \text{ \AA}^{-1}$ , and  $\Delta k = 0.0392 \text{ \AA}^{-1}$ , resulting in  $\alpha_R = 0.41 \text{ eV \AA}^{-1}$ . Contrasting the fit quality of the Zeeman-type splitting, Fig. SM11d shows that  $\mathcal{H}(\{\Sigma''(E_j)\})$  for the optimized RD-type splitting shows large deviations at high  $E_{\text{bin}}$  for the left-hand band and at low  $E_{\text{bin}}$  for the right-hand band. Accordingly, we find  $C = 6.6$  for the Zeeman-type splitting and  $C = 11.2$  for the RD-type splitting, showing that the data points deviate almost twice as far from the model for the RD-type splitting. With the data deviating almost twice as much and visually poor reconstruction, we conclude that the Zeeman-type splitting is predominant over a RD-type splitting of the  $d_{xy}$  bands on the  $\text{TiO}_2$ -terminated surface, although the latter could still be present with weaker magnitude than the Zeeman-type splitting [11].

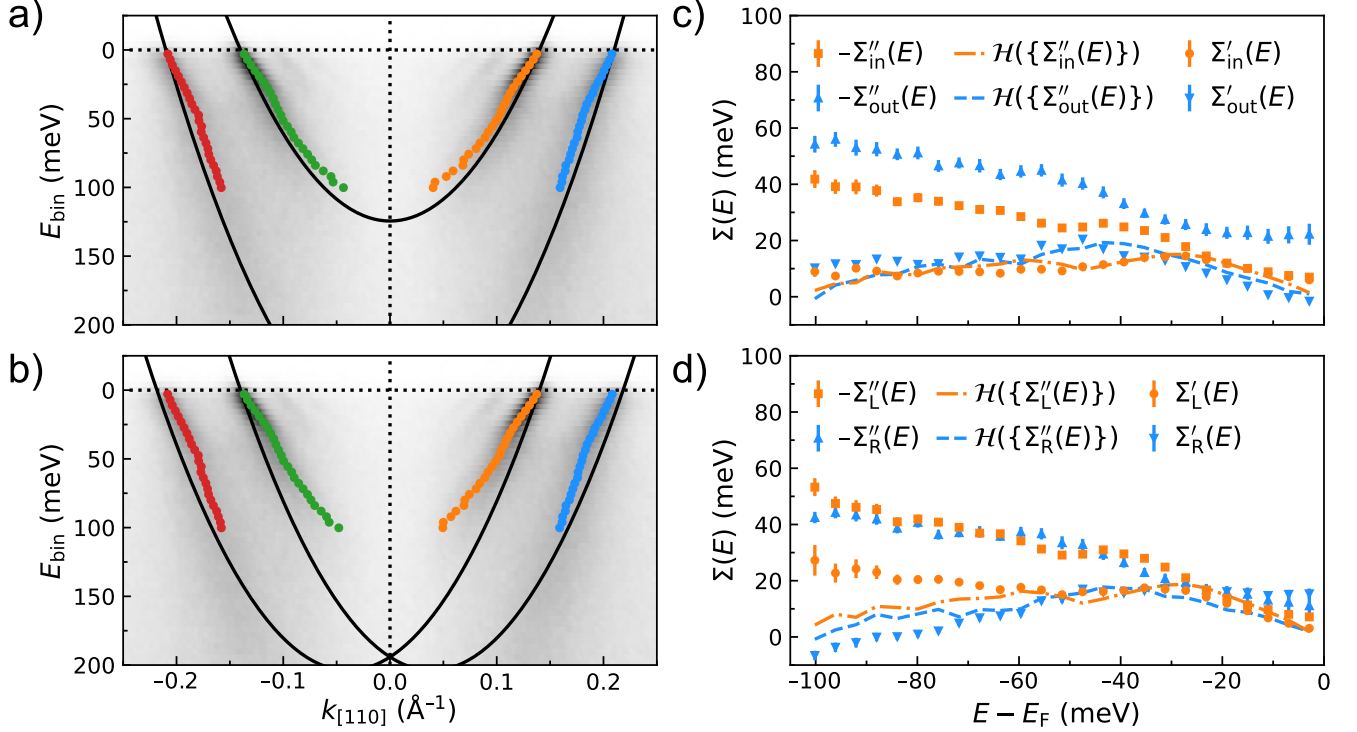

FIG. SM11. **Zeeman- and Rashba-Dresselhaus type splitting of the  $d_{xy}$  bands.** MDC maxima (colored dots) and bare dispersions (black lines) of the  $d_{xy}$  bands on the  $\text{TiO}_2$ -terminated surface according for initial bare band guesses for (a) a Zeeman-type splitting, and (b) a Rashba-Dresselhaus type splitting. The initial guesses for  $m_b$  were determined by visual inspection, whereas  $k_F$  and  $\Delta k$  were determined by setting  $\Sigma'(E = E_F) = 0$ . The optimized  $\{-\Sigma''(E_j)\}$  and the Hilbert transform  $\mathcal{H}(\{\Sigma''(E_j)\})$  compared to  $\Sigma'(E)$  for (c) the inner and outer right-hand branches of the Zeeman-type splitting and (d) the left-and right-hand branches of the right-hand side of the band map for the Rashba-Dresselhaus-type splitting.

## SM9. VIDEO CAPTIONS

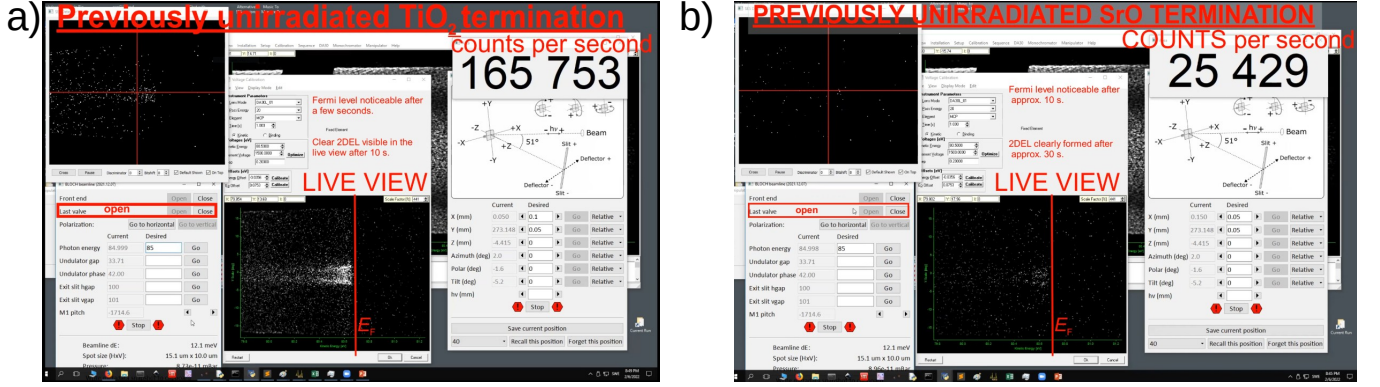

FIG. SM12. Screenshots of the supplemental videos that demonstrate the speed of development for the 2DELs on the two opposite terminations. a) The video titled "TiO<sub>2</sub>-termination\_2DEL\_Time\_evolution\_Screen-recording.avi" shows a real-time recording of a detector live view upon irradiating a previously unirradiated spot on the TiO<sub>2</sub>-terminated surface region of a bulk-terminated SrTiO<sub>3</sub>(001). The surface is first irradiated with 85 eV photons following opening of the last valve in the photon beam line to develop a clear Fermi surface within a few seconds and a clear 2DEL within 10 seconds of irradiation. After the development of a 2DEL, this valve is closed, the photon energy changed to 47 eV, and the valve re-opened to reveal a fully developed 2DEL with lifted orbital degeneracy. b) The video titled "SrO-termination\_2DEL\_Time\_evolution\_Screen-recording.avi" shows a real-time recording of a detector live view upon irradiating a previously unirradiated spot on the SrO-terminated surface region of a bulk-terminated SrTiO<sub>3</sub>(001). Following the opening of the last valve in the photon beam line and irradiating the surface with 85 eV photons, the Fermi level gradually develops and the appearance of a weak 2DEL signal is noticeable after roughly 30 seconds. The intensity and the clarity of this signal increases with increased irradiation. The movies are displayed in real time.

- 
- [1] G. Grimvall, *The Electron-Phonon Interaction in Metals* (North-Holland, Amsterdam, 1981).
  - [2] A. Damascelli, Phys. Scr. **T109**, 61 (2004).
  - [3] Z. Wang, S. M. Walker, A. Tamai, Y. Wang, Z. Ristic, F. Y. Bruno, and F. Baumberger, Nat. Mater. **15**, 6 (2016).
  - [4] C. Berthod, *Spectroscopic Probes of Quantum Matter* (IOP Publishing, 2018).
  - [5] S. Moser, J. Electron Spectrosc. Relat. Phenom. **214**, 29 (2017).
  - [6] H. Iwasawa, E. F. Schwier, M. Arita, A. Ino, H. Namatame, M. Taniguchi, Y. Aiura, and K. Shimada, Ultramicroscopy **182**, 85 (2017).
  - [7] X. P. Yang, H. LaBollita, Z.-J. Cheng, H. Bhandari, T. A. Cochran, J.-X. Yin, M. S. Hossain, I. Belopolski, Q. Zhang, Y. Jiang, N. Shumiya, D. Multer, M. Liskevich, D. A. Usanov, Y. Dang, V. N. Strocov, A. V. Davydov, N. J. Ghimire, A. S. Botana, and M. Z. Hasan, Phys. Rev. B **105**, L121107 (2022).
  - [8] S. Goldberg, C. Fadley, and S. Kono, J. Electron Spectrosc. Relat. Phenom. **21**, 285 (1981).
  - [9] C. S. Kern, A. Haags, L. Egger, X. Yang, H. Kirschner, S. Wolff, T. Seyller, A. Gottwald, M. Richter, U. De Giovannini, A. Rubio, M. G. Ramsey, F. C. Bocquet, S. Soubatch, F. S. Tautz, P. Puschnig, and S. Moser, Phys. Rev. Research **5**, 033075 (2023).
  - [10] P. D. C. King, S. McKeown Walker, A. Tamai, A. de la Torre, T. Eknapakul, P. Buaphet, S.-K. Mo, W. Meevasana, M. S. Bahramy, and F. Baumberger, Nat. Commun. **5**, 3414 (2014).
  - [11] N. C. Plumb, M. Salluzzo, E. Razzoli, M. Månsson, M. Falub, J. Krempasky, C. E. Matt, J. Chang, M. Schulte, J. Braun, H. Ebert, J. Minár, B. Delley, K.-J. Zhou, T. Schmitt, *et al.*, Phys. Rev. Lett. **113**, 086801 (2014).
  - [12] S. Liu, E. Kotta, Y. Xu, J. Mutch, J.-H. Chu, M. Hoesch, S. K. Mahatha, J. D. Denlinger, and L. A. Wray, Journal of Electron Spectroscopy and Related Phenomena **260**, 147255 (2022).
  - [13] A. F. Santander-Syro, F. Fortuna, C. Bareille, T. C. Rödel, G. Landolt, N. C. Plumb, J. H. Dil, and M. Radović, Nat. Mat. **13**, 1085 (2014).
  - [14] S. McKeown Walker, S. Riccò, F. Y. Bruno, A. de la Torre, A. Tamai, E. Golias, A. Varykhalov, D. Marchenko, M. Hoesch, M. S. Bahramy, P. D. C. King, J. Sánchez-Barriga, and F. Baumberger, Phys. Rev. B **93**, 245143 (2016).
  - [15] W. Meevasana, X. J. Zhou, B. Moritz, C.-C. Chen, R. H. He, S.-I. Fujimori, D. H. Lu, S.-K. Mo, R. G. Moore, F. Baumberger, T. P. Devereaux, D. van der Marel, N. Nagaosa, J. Zaanen, and Z.-X. Shen, New J. Phys. **12**, 023004 (2010).
  - [16] T. P. van Waas, C. Berthod, E. B. Guedes, J. Berges, N. Marzari, J. H. Dil, and S. Poncé, (unpublished).
  - [17] R. K. Bryan, Eur. Biophys. J. **18**, 165 (1990).
  - [18] M. Jarrell and J. E. Gubernatis, Phys. Rep. **269**, 63 (1996).
  - [19] C. M. Bishop, *Pattern Recognition and Machine Learning*, Vol. 4 (Springer, 2006).
  - [20] J.-J. Zhou, O. Hellman, and M. Bernardi, Phys. Rev. Lett. **121**, 226603 (2018).
  - [21] T. Jungwirth and A. H. MacDonald, Phys. Rev. B **53**, 7403 (1996).
  - [22] J. Jiang, M. Higashiguchi, N. Tobida, K. Tanaka, S. Fukuda, H. Hayashi, K. Shimada, H. Namatame, and M. Taniguchi, e-J. Surf. Sci. Nanotechnol. **7**, 57 (2009).
  - [23] F. Giustino, Rev. Mod. Phys. **89**, 015003 (2017).
  - [24] A. Eiguren, C. Ambrosch-Draxl, and P. M. Echenique, Phys. Rev. B **79**, 245103 (2009).
  - [25] P. B. Allen and B. Mitrović, Solid State Physics **37**, 1 (1983).
  - [26] G. D. Mahan, *Many-Particle Physics*, 3rd ed., Physics of Solids and Liquids (Kluwer Academic/Plenum Publishers, New York, 2000).
  - [27] H. Vogt, Phys. Rev. B **38**, 5699 (1988).
  - [28] Y. Xie, H.-Y. Cao, Y. Zhou, S. Chen, H. Xiang, and X.-G. Gong, Sci Rep **5**, 10011 (2015).
  - [29] C. Mera Acosta, A. Fazzio, and G. M. Dalpian, npj Quantum Mater. **4**, 41 (2019).
  - [30] C. N. Veenstra, G. L. Goodvin, M. Berciu, and A. Damascelli, Phys. Rev. B **84**, 085126 (2011).
  - [31] I. Pletikosić, M. Kralj, M. Milun, and P. Pervan, Phys. Rev. B **85**, 155447 (2012).
  - [32] R. Noguchi, K. Kuroda, M. Kawamura, K. Yaji, A. Harasawa, T. Iimori, S. Shin, F. Komori, T. Ozaki, and T. Kondo, Phys. Rev. B **104**, L180409 (2021).
  - [33] P. Virtanen, R. Gommers, T. E. Oliphant, M. Haberland, T. Reddy, D. Cournapeau, E. Burovski, P. Peterson, W. Weckesser, J. Bright, S. J. van der Walt, *et al.*, Nat. Methods **17**, 261 (2020).
